# Supplementary material for: Representing Knowledge as Predictions (and State as Knowledge)
Source: arXiv:2112.06336 source file (2021-12-12)
Supplement: Supplementary file 1 [file appendix-locking-in.tex]

\subsection{Locking In}
\label{sec:lockin}
\comment{The appendix is work in progress.}
When a predictive agent receives information that should support its current predictions, how is that information used to bolster its current estimates?
It searches for a stapler in a room and then the stapler gradually comes into view.
At first there is minor evidence that might indicate the presence of the stapler, then more and more, but how is new evidence combined with the evidence seen so far such that the forecast is strengthened, is resilient in the face of noise, and continues when the agent looks away?
We call this the ``locking in'' problem because the evidence should accumulate until the agent is convinced that the stapler is present, at which point, the forecasts regarding the stapler's pattern of interaction are ``locked in,'' and the agent knows that specific ways of interacting have become available.

In the simplest case, the robot has an action (say \FF from Section~\ref{sec:microworld}), that results in an observation (say the signal from the \KU{touch} sensor, $\obs\in\{0,1\}$), and the robot can be in one of two situations: in situation $A$ the robot will touch something if it moves its finger forward, and in situation $B$ it will not.
The sensor is noisy, so if we place the robot facing something that it can touch (e.g., a wall) and it moves its finger forward, there is a probability $P_A$ that it will observe a $1$, and if there is nothing there to touch, then there is a different probability $P_B$ that it will observe a $1$.
How does the agent \emph{decide} at any moment whether it is in state A, where it can reach out and touch something, or state B, where it cannot?
That is, how do its forecasts lock in on the prediction that if it again reaches its finger forward it will (or will not) observe a $1$ through its \KU{touch} sensor?
The forecast is over an option $\{π = \FF, I=1, β=1\}$ whose policy is a single action $\FF$, which can be taken in any state and which always terminates immediately.
The target is $\{\accv=0, \termv=\KU{touch}\}$, which is the value of the touch sensor.
Therefore, the forecast should predict $P(\KU{touch}=1 \mid \FF) \equiv P(1 \mid \action)$, where, for convenience and generality, we use $1$ as an abbreviation for $\KU{touch} = 1$ and $\action$ as the name of the action or option.
But these probabilities should also be contingent on the history of observations in response to this action.
Let $x$ be the most recent sensor observation in response to \action, and let $h$ be the history of all previous sensor observations so far in response to this action, so that $\forecast(\state_t) = P(\KU{touch}=1\mid\FF,h) \equiv P(1\mid h)$, since we are only concerned with that part of the history where the action \FF was taken.
Then,
%
%The belief-state solution to the ``locking in'' problem: in simple case, where x is the first part of string, b is the latest observation, and A is some property of the world:
%
\begin{align*} 
\forecast(\state_t) = P(1 | h) &= P(1|A) P(A| h) + P(1|B) P(B|h) \\
   P(A | hx) &=   \frac{P(hx | A)P_A}{P(hx)} \\
           & =  \frac{P(h | A)P(x | A)P_A}{P(h | A)P(x | A)+P(h | B)P(x | B)P_B} \\
           & =  \frac{\frac{P(A | h) P(h)}{P_A}P(x | A)P_A}
             {\frac{P(A | h)P(h)}{P_A}P(x | A)P_A +
              \frac{P(B | h)P(h)}{P_B}P(x | B)P_B} \\
           & =  \frac{P(A | h)P(x | A)}{P(A | h)P(x | A) + P(B | h)P(x | B)}.
\end{align*}
If the state vector consists of the current observation $x_t$ and the current forecast $\forecast(\statevec_{t-1})$, then this can be rewritten as:
\begin{align*} 
 \forecast(\statevec_{t+1}) = \frac{P(A | h)P(x | A)}{P(A | h)P(x | A) + P(B | h)P(x | B)}.
\end{align*}

\comment{I think it takes a funky 3-layer MLP to calculate this.}
% With a two-layer MLP  whose input vector...
% We assume here a simple linear function approximator for calculating forecasts.
% In this case, $\forecast $
% w=P(A)
% Assuming that the forecast estimate is correct, then $\forecast(A) = P_A$, so 
%
\begin{align*} 
 P(1 | h) &= P(A| h)P_A + P(B | h) P_B\\
 P(1 | h) &= P(A| h)w_A + P(B | h) w_B\\
   P(A | ho) &=   \frac{P(ho | A)w_A}{P(ho)} \\
           & =  \frac{P(h | A)P(o | A)w_A}{P(h | A)P(o | A)+P(h | B)P(o | B)w_B} \\
           & =  \frac{\frac{P(A | h)P(h)}{w_A}P(o | A)w_A}
             {\frac{P(A | h)P(h)}{w_A}P(o | A)w_A +
              \frac{P(B | h)P(h)}{w_B}P(o | B)w_B} \\
           & =  \frac{P(A | h)P(o | A)}{P(A | h)P(o | A) + P(B | h)P(o | B)}
\end{align*}

And similarly for $P(B|ho)$.
Figure~\ref{fig:lockin-simple} shows a sample interaction for the value of $P(1 | h)$ when the agent is in situation $A$ and $P_A = 0.9$, and also when $P_A = 0.8$.

The picture is more complex than this, however, in that there is always some chance that the robot's situation might change and then its forecast must also change.
Say the probability of switching from situation A to situation B is P(switch), then 
\begin{align*} 
  P(A | ho)  = & (1-P(switch)) * \frac{P(A | h)P(o | A)}{P(A | h)P(o | A) + P(B | h)P(o | B)} \\
          &    + P(switch) *  \frac{P(B | h)P(o | A)}{P(B | h)P(o | A) + P(A | h)P(o | B)}
\end{align*}
Because there is some chance that no switch has occurred (first line), in which case the calculation would be as in the simple case, and there is some chance that a switch has occurred (second line), in which case the previous $P(B | h)$ and $P(A | h)$ values were reversed, so should be handled in reverse.
The overall update just is the first case, multiplied by its chance of occurrence plus the second case, multiplied by its chance of occurrence.

In the same way, any perception becomes substantiated by evidence. Consistent pieces of evidence will be mutually reinforcing. Figure~\ref{fig:lockin-switch} shows an interaction in which the robot changes from situation A to situation B, with the same probabilities far $P_A$ as in the previous graph. 

\commentout{
Important:
  . learning these things -- i.e., learning the answers -- can involve all the
    sensory information where it isn't necessary to know what the relationships
    would be, e.g., using visual information to learn what a doorway looks
    like, though it is not ``defined'' in terms of visual information.
    . now, how can that ``answer'' be used then to help define the question?
  . the answer net itself is responsible for defining values that ``lock in''
    to concepts so that their relationships are known.
    . in the same way, an ``unknown'' environment can become ``known'' through
    lock in only, i.e., just by state estimation where ``unknown'' becomes
    ``known'' and these are represented explicitly enough that the transition
    from one to the other is just part of the state.
}

%%% Local Variables: 
%%% mode: latex
%%% TeX-master: "predictive representations of state and knowledge"
%%% End: 
